# Supplementary material for: AeroScene: Progressive Scene Synthesis for Aerial Robotics
Source: arXiv:2603.23224 source file (2026-04-18)
Supplement: Supplementary file 1 [file 6_appendix.tex]

\section*{APPENDIX}

\subsection{Convergence Analysis of $\mathcal{L}_{\rm {cd^+}}$}
It is typical in deep learning to hold the learning rate constant and only decay it when the learning process saturates. As a result, we give the analysis for the fixed learning rate situation and investigate how $\mathcal{L}_{\rm {cd^+}}$ interacts with the optimizer DPSGD~\cite{wang2018cooperative}.

% Under the Siamese setup, DPSGD is formed as a multi-task updater. Reminded from the paper, at each iteration $k$, the update in the backbone for $\mathcal{L}_{\rm {cd^+}}$ is described as: 
% \begin{equation}
% \begin{aligned}
%  &\theta^b_i\left(k + 1\right) \\
%  & =\begin{cases}
%     \sum_{j \in \mathcal{N}_i^{+} \cup{\{i\}}}\textbf{A}_{i,j}{\theta}^b_{j}\left(k\right), \textit{ \quad \quad \quad if k} \equiv 0 \pmod{s + 1},\\
%     {\theta}^b_i\left(k\right)-\alpha_{k}\frac{1}{m}\sum^m_{h=1}\nabla \mathcal{L}_{\rm {lr^+}}\left({\theta}^b_i\left(k\right),\xi_i\left(k\right)\right),  \text{otherwise.}
% \end{cases}
% \end{aligned}
% \label{eq:ori_backbone_DFL}
% \end{equation}
% where $\mathcal{L}_{\rm {lr^+}} = \mathcal{L}_{\rm {lr}} + \mathcal{L}_{\rm {cd^+}}$ 
% where $m$ is the mini-batch size and $\alpha_k > 0$ is a potentially varying learning rate.

% In parallel,  the updates in sub-network are described at each iteration $k$ as:

% \begin{equation}
% \begin{aligned}
%  &\theta^s_i\left(k + 1\right) ={\theta}^s_i\left(k\right)-\alpha_{k}\frac{1}{m}\sum^m_{h=1}\nabla \mathcal{L}_{\rm {cd^{-}}}\left({\theta}^s_i\left(k\right),\xi_i\left(k\right)\right)
% \end{aligned}
% \label{eq:ori_support_DFL}
% \end{equation}

% While the learnable parameters of the backbone follow the original update rule of the DPSGD and the positive term of CD (Eq.~\ref{eq:ori_backbone_DFL}), the CD regularizer updates corresponds to replacing the update term of the sub-network (Eq.~\ref{eq:ori_support_DFL}). 

\textbf{Assumptions.} The analysis is carried out under the following assumptions, which are similar to those used in prior research on distributed SGD analysis~\cite{wang2018cooperative, wang2019slowmo, koloskova2020unified, moreau2021dpsgd}.
\begin{enumerate}
    \item (Unbiased gradients): $\mathbb{E}_{\xi|x}[g(x)] = \nabla F(x)$
    \item (Smoothness): $||\nabla F(x)-\nabla F(x')|| \leq \mathbf{L}||x-x'||$
    \item (Lower bounded): $F(x) \geq F_{inf}$
    \item (Bounded variance): $\mathbb{E}_{\xi|x}||g(x)-\nabla F(x)||^2 \leq \omega||\nabla F(x)||^2 +\sigma^2$ where $\omega$ and $\sigma^2$ are non-negative constants and in inverse proportion of the mini-batch size $m$.
    \item (Mixing Matrix): $\mathbf{W}\mathbf{1}_{m+v} = \mathbf{1}_{m+v}, \mathbf{W}^T = \mathbf{W}$. All eigenvalue magnitudes $\lambda$ except the largest one are strictly less than 1: $max\{| \lambda_2\mathbf{W}|,| \lambda_{m+v}\mathbf{W}|\} < \lambda_1(\mathbf{W}) = 1$
\end{enumerate}
where $F(.)$ is the hypothesis of $\theta^b_i$; $\mathbf{L}$ is Lipschitz constant; $g(x)$ is Stochastic gradients.

\textbf{Convergence Analysis.} 
For all algorithms that follow $A(\tau,\mathbf{W}, v)$ form (including the update rule for backbone in Equation~\ref{eq:ori_backbone_DFL}), suppose the total number of iterations $K$ can be divided by the communication period $\tau$. Under Assumptions $1–5$ (with $\omega = 0^2$), as in~\cite{wang2018cooperative}, if the learning rate satisfies:
\begin{equation}
\small
\begin{aligned}
\alpha_e\mathbf{L} + 5\alpha_e^2\mathbf{L}^2\left[\left(1+\frac{v}{N}\right)\frac{\tau}{1-\zeta}\right]^2\leq 1
\end{aligned}
\label{eq:lr_const}
\end{equation}
where $\zeta = max\{| \lambda_2\mathbf{W}|,| \lambda_{m+v}\mathbf{W}|\}$ is the second largest absolute eigenvalue; $\alpha_e= \frac{N}{N+v}\alpha$ is the effective learning rate;  $v$ is the number of auxiliary variables; and all local
models are initialized at a same point $\mathbf{u}_1$. Then, the average squared gradient norm after $K$ total iterations is bounded as:
\begin{equation}
\footnotesize
\begin{aligned}
&\mathbb{E}\left[\frac{1}{K} \sum^{K}_{k=1}{||\nabla F(\mathbf{u}_k)||^2}\right] \leq \\
& \frac{2\left[F(\mathbf{u}_1)-F_{inf}\right]}{\alpha_e K}v  + \frac{\alpha_e \mathbf{L} \sigma^2}{m} + \alpha_e^2 \mathbf{L}^2 \sigma^2\left(\frac{1 + \zeta^2}{1-\zeta^2}\tau -1\right)\left(1+\frac{v}{N}\right)^2 \\
&\xrightarrow{K\rightarrow \infty}  \frac{\alpha_e \mathbf{L} \sigma^2}{m} + \alpha_e^2 \mathbf{L}^2 \sigma^2\left(\frac{1 + \zeta^2}{1-\zeta^2}\tau -1\right)\left(1+\frac{v}{N}\right)^2
\end{aligned}
\label{eq:norm_bound}
\end{equation}
where $\mathbf{u}_k=\mathbf{X}_k\frac{\mathbf{1}_{N+v}}{N+v}$ is the aggregated model for updating at $k$-th round; $\mathbf{X}_k \in \mathbb{R}^{d \times (N \times v)}$ is the defined matrix concatenating all local models and gradients at $k$-th round; $d$ is the feature dimension.
\subsection{Inference Scheme}
% As in SFL setup~\cite{mcmahan2017communication}, to compute the prediction of models in all silos, they compute the average model $\theta$ using weight aggregation from all the local model $\theta_i$. However, in DFL, we focus on the case when not always all silos are available for averaging at the same time. Besides, test samples can be shared between local silos. Thus, 
Following Federated Boosting (FedBoost~\cite{hamer2020fedboost}), we first compute the predictions of test samples internally at each silo. Then, based on the connection of all notes at test time, we aggregate the results. 
% Note that, this technique is modified to adapt to the autonomous driving scenario and regression task. 
FedBoost is conducted as follows:

\begin{equation}
\eta(\iota) = \frac{1}{\sum^N_{i=0}{\vartheta_i}} \sum^N_{i=0}\vartheta_i \eta_i(\theta^b_i,\iota)
\label{eq:aggr_model}
\end{equation}
where $N$ is the number of silos; $\vartheta_i = \{0,1\}$ is the aggregation status. $\vartheta_i = 1$ indicates that silo $i$ joins the inference process and $\vartheta_i = 0$ if not. The boosted prediction $\eta$ of an input sample $\iota$ in the test set $\mathcal{D}_{test}$ is then used for evaluation.
